# Supplementary material for: Generating High Fidelity Data from Low-density Regions using Diffusion Models
Source: arXiv:2203.17260 source file (2022-06-26)
Supplement: Supplementary file 2 [file appendix.tex]

\section{Appendix}
You may include other additional sections here.

\subsection{Using $64\times64$ image resolution.}
While we will provide our final results with the standard $224\times224$ resolution images, we do conduct our major analysis and ablation studies with the $64\times64$ image resolution. This is because sampling high resolution images from diffusion model is highly computationally expensive (provide quantitative numbers). But we argue that using low resolution doesn't change our results. For examples, training on synthetic data from imagenet100 on both resolutions leads to 79-80\% accuracy on real data. Not much difference. 

TODO:
\begin{itemize}
    \item Some classes respond more strongly that other with scaling of hardness loss, since the accuracy of these classes degrades quickly to zero. Even with scaling, these classes have less accuracy than real data classes, showing that ddpm model is not learning the correct mode. Also if the accuracy degrades so quickly, it mean that mode volume is also not large, i.e., long tail is not modelled correct by the distribution. Rather than just saying that we discard classes, we should highlight this phenomenon very clearly. One other way is to add the real-synthetic distribution scatter plot with increasing hardness score, as that can better clarify which classes degrades heavily with increasing hardness. 
    tl;dr; Not classes more modelled equally well by generative model and they further don't behave equally under hardness optimization. 
    \item Another interesting question is why we don't end up with adversarial examples. Since we use gradients of loss, which are basically going to create adversarial examples. But they don't. Why? Now note that while we don't run into pixel-perturbation based adversarial examples, the sampling mechanism can exploit some other biases of classifier to satisfy the objective (in very few cases). This includes changing the background of the images, changing color etc. 
    \item Language models are known to memorize low density samples. So is it the same thing happening here too. Give visualization and some concrete evidence (i.e., distance to nearest five neighbors). 
    \item When selecting classes for the ImageNet400 model, provide a class-wise plot showing that some classes are indeed very hard to model even for the best generative model, thus most of their samples aren't correctly classified. Plot the classification output itself. Since these classes even in uniform setting don't generate very accurate samples, it quite hopeless to assume that our method will do much on them, i.e., uniform sampling itself generates hardness samples. 
    \item 
\end{itemize}


\begin{figure}
    \centering
    \includegraphics[width=0.8\linewidth]{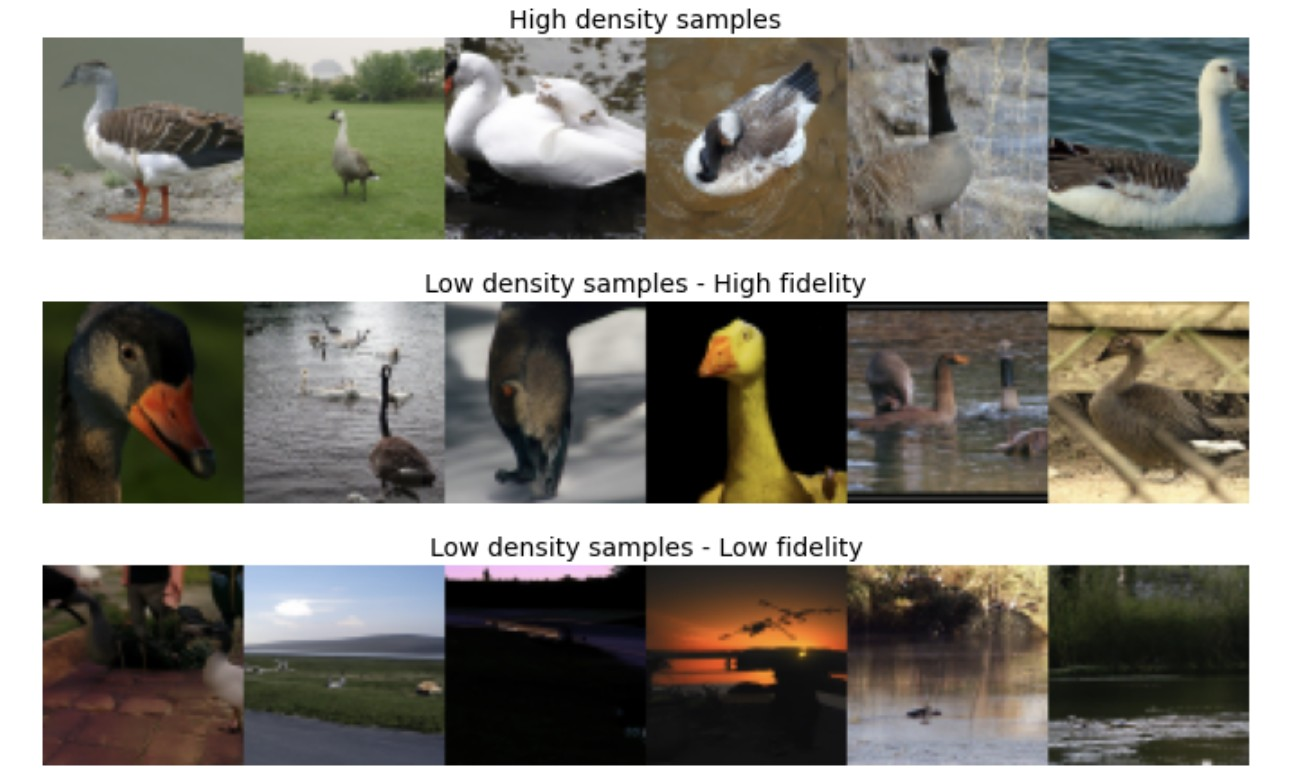}
    \caption{\textbf{Why we need to improve image fidelity?}}
\end{figure}
